# Supplementary material for: The domain wall spin torque-meter
Source: arXiv:0810.4633 source file (2008-10-25)
Supplement: Supplementary file 1 [file supplementarynotes_Miron.pdf]

## Experimental details

Samples are fabricated from magnetron sputtered films of $Pt_{3nm}Co_{0.6nm}Pt_{3nm}$ and $Pt_{3nm}Co_{0.6nm}(AlO_x)_{2nm}$.

The thin films are patterned by electron beam lithography and Ar ion etching.

For the Hall Effect measurements we have used a high resolution NI : PXI4461 acquisition card. The temporal signals were measured at a rate of 24ksamples/s. The measurement scale was set to 0.1 V, while the acquisition card has a 24bit resolution.

The current is injected using an analog voltage output of the same acquisition card in series with the sample and a resistance of 20 kΩ. As the electrical resistance values of the samples are much smaller ~ 2 kΩ and practically do not vary during the measurement, this setup can be considered as a perfect current source. The only variations of the resistance are due to changes in the Hall resistance which is of the order of 1 Ω.

We apply an alternative low frequency (10 Hz) current for 10 seconds (100 periods), measure the temporal AHE signal and then compute the corresponding Fast Fourier Transform (FFT). We repeat the measurement and average the FFTs, until the noise level of the FFT dimishes close to 5 nV (typically 10 to 20 times).

The harmonicity of the injected current is checked by comparing the output voltage with the voltage across the sample (on the wire where the current is passed) during the current injection. The ratio between the current at the frequency $2f$ and the one at $f$ was found to be smaller than $10^{-6}$. This ratio has the same value both for the signal delivered by the voltage source and for the voltage measured across the sample. This means that this $2f$ signal is entirely caused by nonlinearities of the voltage source. Note

that as the inharmonicity of the applied current was found ~$10^{-6}$ it will cause a *2f* voltage of around 0.1 nV, smaller than the noise level.

The magnetic field is applied using a pair of Helmholtz coils powered by a commercial Kepco current source. The Kepco current source is controled by a second voltage output of the same acquisition card. All measurements were done at room temperature.

The Hall resistance is about 1 Ω for the Pt/Co/$AlO_x$ samples and around 0.5 Ω for the Pt/Co/Pt samples. This corresponds to the change in the measured resistance when the magnetization is switched. The maximum injected current amplitude is around 150 μA. In this case the voltage amplitude will be 150 μV. As the minimal detectable voltage change is of the order of the noise level, the minimal detectable resistance change is of the order of 0.06 mΩ. If the sensitivity to DW motion of the Hall cross is homogeneous, we estimate that the ratio between the total surface of the Hall cross and the area that switches when the DW moves, should be equal to the ratio between the total Hall resistance and the respective resistance variation. As the approximate lateral size of the cross is around 100 nm and the above mentioned ratio is close to $1\cdot 10^4$ we estimate that using this measurement protocol, the magnetic switching of a surface of about 1 $nm^2$ can be detected. Supposing that in the case of small displacements the reversed surface is distributed homogeneously along the DW, the 1 $nm^2$ would correspond to an average DW displacement of 10 pm.

The domain wall is prepared on the constriction by scanning the sample with a magnetic force microscope tip magnetized opposed to the samples magnetization. The

tip's stray field is strong enough to nucleate a domain and then to drag the DW through the wires.

The positioning of the DW on the constriction is verified directly by transport measurements. A cross should be almost saturated upwards while the other should be almost saturated downwards.

The resistance of a Hall cross has two components: the Hall resistance $R_H$ which depends on the local magnetization, and the longitudinal resistance $R_0$ due to the misalignment of the two lateral wires, which does not depend on the local magnetization $R = R_0 \pm R_H$. As the FFT only gives the amplitude of the frequency components it is not always possible to obtain the value of the Hall resistance by subtracting the saturated up to the saturated down resistance. If the longitudinal component is smaller than the Hall component, the resistance will change sign upon magnetization reversal. In this case, it is the sum of the two values obtained from the FFT for the saturate states that will yield the value of the Hall resistance. This problem can be easily overcome by comparing the signs of the two resistances directly from the measured temporal signals.

**Spintorque on a DW. The LLG equation.**

The non-adiabatic term of the spin torque was simultaneously introduced by Thiaville et al.[7] and calculated by Zhang and Li[6] within a framework of a semiclassical transport theory. Vanhaverbeke and Viret[17] had a different approach based on the Larmor precession of the conduction electrons around the local s-d exchange field, but also found a similar expression. Further on we will use the extended Landau Lifshitz Gilbert (LLG) equation in the form that was proposed by Zhang and Li[6].

$$\frac{\partial M}{\partial t} = \gamma M \times H_{eff} + \frac{\alpha}{M_S} M \times \frac{\partial M}{\partial t} - \frac{b_j}{M_S^2} M \times \left( M \times \frac{\partial M}{\partial x} \right) - \frac{c_j}{M_S} M \times \frac{\partial M}{\partial x} \quad (1)$$

Here $b_j = Pj_e\mu_B / eM_S(1+\xi^2)$ (2), and $c_j = Pj_e\mu_B\xi / eM_S(1+\xi^2)$ (3), where $P$ is the spin polarization of the electric current, $j_e$ the current density, $\mu_B$ the Bohr magneton, $e$ the electronic charge, $M_S$ the saturation magnetization and $\xi = \tau_{ex}/\tau_{sf}$ the ratio between the exchange and spin-flip characteristic times. Note that this coefficient is the same as β (used in the article), the coefficient generally used to designate the strength of the non-adiabatic component of the spin torque with respect to the adiabatic one.

When the current induced displacement equals the field induced displacement, the values of the two applied torques, integrated on the wall volume are the same.

$$\frac{1}{d}\int_d \frac{c_j}{M_S}\vec{M}\times\frac{\partial\vec{M}}{\partial x}\,dx = \frac{1}{d}\int_d \gamma\,\vec{M}\times\vec{H}_Z\,dx \qquad (4)$$

For simplicity of calculations we will assume that the angle of rotation of the magnetization inside the DW varies linearly. In this case, the non-adiabatic coefficient yields:

$$c_j = \gamma H_Z \frac{2d}{\pi^2} \qquad (5)$$

$$\frac{Pj_e\mu_B}{eM_S}\frac{\xi}{(1+\xi^2)} = \gamma H_Z \frac{2d}{\pi^2} \qquad (6)$$

Both the $Pt_{3nm}Co_{0.6nm}(AlO_x)_{2nm}$ and $Pt_{3nm}Co_{0.6nm}Pt_{3nm}$ layers have a measured magnetic anisotropy field $H_a = 8\ kOe$. By considering an approximate exchange constant[7] $A \approx 10^{-11}$ J/m we estimate that the DW width $d \approx 4.2nm$, where $d = \sqrt{A/K}$ and $K = \frac{1}{2}\mu_0 M_S H_a$.

The current to field correspondence was measured to be 1.25 $10^5$A/cm$^2$ for 1Oe in the case of $Pt_{3nm}Co_{0.6nm}(AlO_x)_{2nm}$ samples. By replacing these values in the above equation (6), we obtain two possible values for the nonadiabacity parameter $\xi_1 \approx \frac{1}{3}$ and $\xi_2 \approx 3$. Note that these estimations were done for a polarization value P=1. A smaller value for the polarization would yield two values of β closer to 1. For example when the polarization is consider to be P=0.6, the quadratic equation will only have one solution $\xi_{1,2} = 1$.

A scenario of momentum transfer[27] to the DW is ruled out by the small nonadiabacity parameter obtained for the Pt/Co/Pt layers.

In this case, in order to have the effect of a field of 1 Oe on the DW, a current density bigger than $5 \cdot 10^6$ A/cm$^2$ is needed. The same estimations yield for $\xi$ in this case a value smaller than 0.02.

**Thermal effects: Joule heating and the Nernst-Etthingshaussen Effect.**

The most commonly encountered thermal effect, when passing a current through a metal, comes from the Joule heating. As the resistance varies as an even function of current, the voltage will vary at twice this frequency (*2f*) and therefore will generate a voltage at *3f*.

Because the lateral contacts are never perfectly aligned, the resistance we measure has in addition to the transverse component created by the AHE a longitudinal one. The effect of the heating (3f peak) will also have two components.

In order to estimate the average temperature of the sample, we take the sum of the FFTs of the temporal signal (supplementary figure 2) corresponding to the two saturated

states and divide it by 2. This way the contribution from the AHE resistance is removed. The comparison of the peak at 3*f* with the one at *f* yields the value of the relative resistance variation of the longitudinal component of the resistance. As most of the current goes through the Pt layer we consider that taking the Pt temperature coefficient of resistance (0.00392) is a good approximation. This way we estimate that the increase of the average temperature due to joule heating is approximately 0,25 K for a current density of 2,5 $10^7$ A/cm$^2$ . This small value can be explained by the relatively small injected current and by the shape of our device.

While in the case of a long and narrow wire the heat created all along the wire is slowly evacuated through the ends of the wire, in our case the existence of the four contacts so close to the constriction allows much faster cooling.

Although the average joule heating is found to be small (insufficient to decrease significantly the depinning field,) the temperature gradients can be relatively high, as the distance over which the temperature variations occur is very small (~100 nm, the lateral size of a hall cross).

While the Joule heating is related to the average sample temperature, in materials showing an important AHE another effect caused by temperature gradients can become important. The Nernst-Ettingshausen Effect (NEE) predicts that a voltage would be created perpendicularly both to the temperature gradient and the magnetization. As the current in the region of the Hall crosses is inhomogeneous, a thermal gradient can appear in the same direction as the passing current and create a transverse voltage, similarly to the AHE. The temperature gradient is proportional to the average temperature, so the

output voltage will be an even function of current. As a result, it will vary at a frequency *2f* and will have an amplitude proportional to $I^2$.

Indeed we have observed the existence of a *2f* signal in the saturated state. Similarly to the AHE this effect is changing sign as the magnetization is reversed, and depends on the DW position. This sign change is not directly visible on the FFT of the measurement, as it only causes a phase inversion of the *2f* signal.

In order to check the phase inversion specific to the NEE we add a small *2f* component to the injected current. If this component is in phase with the NEE the total amplitude of the *2f* voltage will increase. By comparing for the saturated states the value of the *2f* signal with and without the injected *2f* current we have observed the phase inversion and confirm the NEE scenario.

In order to bring further evidence of the thermal nature of this effect, we have fabricated highly asymmetrical samples where one side of the wire was much narrower. This way we have increased the thermal gradient inside one of the two Hall crosses. As expected we have noticed a big increase of the *2f* component corresponding to the "hotter" cross.

**Effects of the Oersted field.**

The pinning of the DW inside the wire can be modeled by a perpendicular field that is zero for the center of the pinning position. The Oersted field has a highly non-uniform perpendicular component. Adding this component to the effective pinning field could in principle change the local energy landscape and thus the pinning. Further on we will show that in our case this contribution is negligible using symmetry arguments and order of magnitude considerations.

The utmost value of the perpendicular component of the Oersted field is reached on the edges of the wire, but it rapidly decreases towards the center. This perpendicular component of the Oersted field is anti-symmetric with respect to the center of the wire: on one side of the wire it is positive while on the other it is negative.

In the case where the pinning of the DW is symmetric the net effect of the Oersted field is zero, as it averages out on the length of the DW.

As the pinning is random, one could assume that generally it is asymmetric. But if this asymmetry arises from the random character it should be different for the different Pt/Co/AlO samples and the effect should be similar for the Pt/Co/Pt samples. In return, we observe the same current-field equivalence on several Pt/Co/AlO samples and no effect on the Pt/Co/Pt ones.

We estimate that the Oersted field can reach a maximum value of ~10 Oe on the edge of the wire for the maximum current that we inject. Note that its value is decreasing very fast: at just 4 nm from the edge its value goes down to ~5 Oe.

In our measurements we have observed a current to field equivalence of 1.25 $10^5$A/cm$^2$ for 1Oe, while the current to field correspondence due to the Oersted field is 2.5 $10^6$A/cm$^2$ to 1Oe. This high value shows that even if the pinning is asymmetric and if the Oersted field has a contribution to the displacement, it can not account to the magnitude of this effect. It can only add a small error (~ 5% ) to the accuracy of the torque measurement.

**Supplementary References:**

27 Tatara, G. & Kohno, H. Theory of current-driven domain wall motion: Spin transfer versus momentum transfer. *Phys. Rev. Lett.* **92,** 086601 (2004).

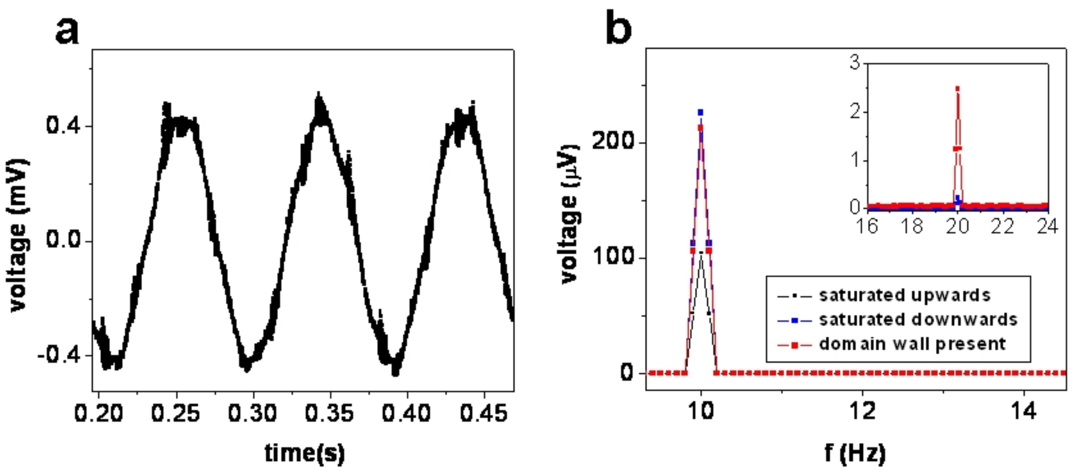


**Supplementary figure 1. Example of measurements on a Pt/Co/AlOx sample.**

**a,** Example of a temporal measurement for a saturated downwards state. In this case the applied current amplitude was 100μA. **b,** The FFT for the three magnetic configurations: The peak observed at the same frequency as the applied current measures the average value of the resistance. The inset zooms on the *2f* signals on the FFT. The curves corresponding to the saturated states (black and blue) show much smaller amplitude at *2f*.

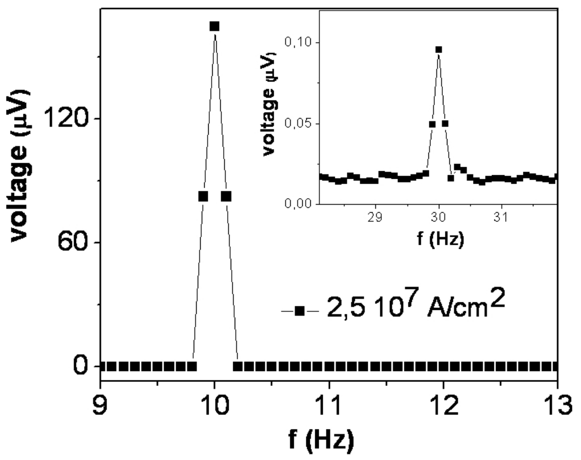


**Supplementary figure 2. The thermal effects: Joule heating**

Example of the average of the FFTs of the temporal signal corresponding to the two saturated states. The small ratio between the 3f (see inset) and the f component of the signal is very small ~ $10^{-3}$ indicating that the change of the temperature caused by the current is also small.

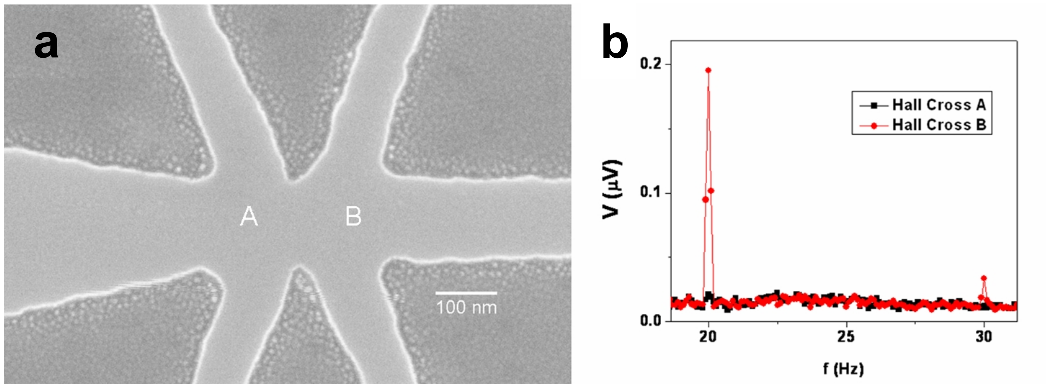


**Supplementary figure 3. The thermal effects: the NE effect**

**a,** A SEM image of the asymmetric sample. **b,** An example of the measurement done in a magnetically saturated state for a current amplitude of 100μA and a current frequency of 10Hz. It is clear that the Hall cross B is hotter, as the *2f* and *3f* voltages have a much higher amplitude.

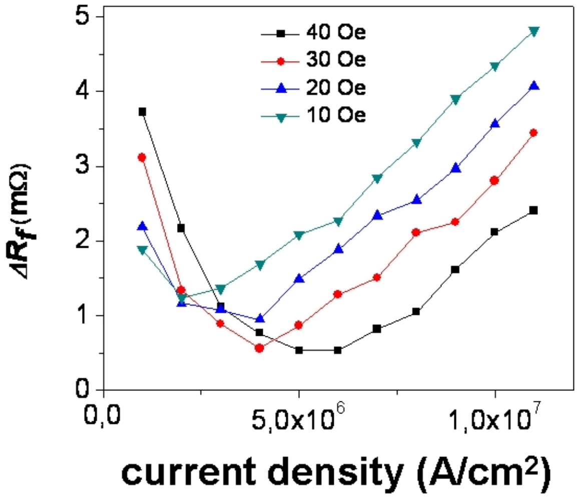


**Supplementary figure 4.** The resistance variation at the frequency of the current for small current and field amplitudes. The fact that we use the injected current to detect the displacements imposes its limits: smaller values of current produce a signal with a lower signal to noise ratio. Despite this limitation, it is clear that the field to current correspondence is the same down to the lowest current values.
